# Supplementary material for: AndroidGen: Building an Android Language Agent under Data Scarcity
Source: arXiv:2504.19298 source file (2025-04-27)
Supplement: Supplementary file 1 [file androidworld.tex]

\section{Details of AndroidWorld Dataset}
In our evaluation (shown in Section~\ref{exp:androidworld}), the AndroidWorld dataset comprises 17 apps and 91 test cases. Due to environmental error issues, we excluded the \texttt{RecipeDelete} and \texttt{Calendar} test samples. 
The data distribution is in Figure~\ref{fig:testset_proportion}.

\begin{figure}[h!]
     \centering
    \vspace{-8mm}
    \includegraphics[width=\linewidth]{images/testset_destribution.pdf}
    \vspace{-17mm}
   \caption{AndroidWorld Data Distribution.}
   \vspace{-5mm}
   \label{fig:testset_proportion}
\end{figure}
